# Supplementary material for: The Shape of the Cosmic X-ray Background: Nuclear Starburst Discs and the Redshift Evolution of AGN Obscuration
Source: arXiv:1711.05268 source file (2018-01-08)
Supplement: Supplementary file 1 [file appendices.tex]

%\section{Appendicies}
\subfile{appendices/rmo}
